# Supplementary material for: Generative Adversarial Networks for Extreme Learned Image Compression
Source: arXiv:1804.02958 source file (2019-08-18)
Supplement: Supplementary file 1 [file fig_appendix_cityscapes_base.tex]

OUTDIR=fig_appendix_cityscapes
{\setlength{\tabcolsep}{1pt}
\begin{tabular}{rccl}
&Ours&BPG\\
\rotatebox[origin=c]{90}{BPP0 bpp}&
\raisebox{-0.5\height}{\includegraphics[width=0.45\linewidth]{https://people.ee.ethz.ch/~aeirikur/pix2bits_results/label2city_512p_globalcompression_mse10_4ch_nolabels250918_cityscapes20perchannel/test_50/images/frankfurt_000000_011074_leftImg8bit_0.03641bpp_synthesized_image.jpg O=ours1}} &
\raisebox{-0.5\height}{\includegraphics[width=0.45\linewidth]{https://data.vision.ee.ethz.ch/mentzerf/user_study_extreme/cityscapes20/frankfurt_000000_011074_real_image_bpg_48_0.0397.png O=bpg1}}&
\rotatebox[origin=c]{90}{BPP1 bpp}\vspace{2pt} \\
\rotatebox[origin=c]{90}{BPP2 bpp}&
\raisebox{-0.5\height}{\includegraphics[width=0.45\linewidth]{https://people.ee.ethz.ch/~aeirikur/pix2bits_results/label2city_512p_globalcompression_mse10_4ch_nolabels250918_cityscapes20perchannel/test_50/images/frankfurt_000000_022797_leftImg8bit_0.03577bpp_synthesized_image.jpg O=ours2}} &
\raisebox{-0.5\height}{\includegraphics[width=0.45\linewidth]{https://data.vision.ee.ethz.ch/mentzerf/user_study_extreme/cityscapes20/frankfurt_000000_022797_real_image_bpg_51_0.0385.png O=bpg2}}&
\rotatebox[origin=c]{90}{BPP3 bpp}\vspace{2pt} \\
\rotatebox[origin=c]{90}{BPP4 bpp}&
\raisebox{-0.5\height}{\includegraphics[width=0.45\linewidth]{https://people.ee.ethz.ch/~aeirikur/pix2bits_results/label2city_512p_globalcompression_mse10_4ch_nolabels250918_cityscapes20perchannel/test_50/images/frankfurt_000001_010156_leftImg8bit_0.03577bpp_synthesized_image.jpg O=ours3}} &
\raisebox{-0.5\height}{\includegraphics[width=0.45\linewidth]{https://data.vision.ee.ethz.ch/mentzerf/user_study_extreme/cityscapes20/frankfurt_000001_010156_real_image_bpg_51_0.0428.png O=bpg3}}&
\rotatebox[origin=c]{90}{BPP5 bpp}\vspace{2pt} \\
\rotatebox[origin=c]{90}{BPP6 bpp}&
\raisebox{-0.5\height}{\includegraphics[width=0.45\linewidth]{https://people.ee.ethz.ch/~aeirikur/pix2bits_results/label2city_512p_globalcompression_mse10_4ch_nolabels250918_cityscapes20perchannel/test_50/images/frankfurt_000001_017101_leftImg8bit_0.03589bpp_synthesized_image.jpg O=ours4}} &
\raisebox{-0.5\height}{\includegraphics[width=0.45\linewidth]{https://data.vision.ee.ethz.ch/mentzerf/user_study_extreme/cityscapes20/frankfurt_000001_017101_real_image_bpg_50_0.0370.png O=bpg4}}&
\rotatebox[origin=c]{90}{BPP7 bpp}\vspace{2pt} \\
\rotatebox[origin=c]{90}{BPP8 bpp}&
\raisebox{-0.5\height}{\includegraphics[width=0.45\linewidth]{https://people.ee.ethz.ch/~aeirikur/pix2bits_results/label2city_512p_globalcompression_mse10_4ch_nolabels250918_cityscapes20perchannel/test_50/images/frankfurt_000001_029236_leftImg8bit_0.03621bpp_synthesized_image.jpg O=ours5}} &
\raisebox{-0.5\height}{\includegraphics[width=0.45\linewidth]{https://data.vision.ee.ethz.ch/mentzerf/user_study_extreme/cityscapes20/frankfurt_000001_029236_real_image_bpg_51_0.0446.png O=bpg5}}&
\rotatebox[origin=c]{90}{BPP10 bpp}\vspace{2pt} \\
\end{tabular}}
