# Supplementary material for: Generative Adversarial Networks for Extreme Learned Image Compression
Source: arXiv:1804.02958 source file (2019-08-18)
Supplement: Supplementary file 2 [file fig_appendix_kodak_base.tex]

OUTDIR=fig_appendix_kodak
{\setlength{\tabcolsep}{1pt}
\begin{tabular}{rccl}
&Ours&BPG\\
\rotatebox[origin=c]{90}{BPP0 bpp}&
\raisebox{-0.5\height}{\includegraphics[width=0.45\linewidth]{https://people.ee.ethz.ch/~aeirikur/pix2bits_results/openimages_GC_60ch_NL_MSE10_BN4_LEVELS5no_IN200918_kodakperchannel/test_iter_140000/images/kodim01_0.03369bpp_synthesized_image.jpg O=ours1}} &
\raisebox{-0.5\height}{\includegraphics[width=0.45\linewidth]{http://people.ee.ethz.ch/~mentzerf/pix2bits_results/bpg/kodak_bpg/kodim01_bpg_50_0.0433.png O=bpg1}}&
\rotatebox[origin=c]{90}{BPP1 bpp}\vspace{2pt} \\
\rotatebox[origin=c]{90}{BPP2 bpp}&
\raisebox{-0.5\height}{\includegraphics[width=0.45\linewidth]{https://people.ee.ethz.ch/~aeirikur/pix2bits_results/openimages_GC_60ch_NL_MSE10_BN4_LEVELS5no_IN200918_kodakperchannel/test_iter_140000/images/kodim02_0.03046bpp_synthesized_image.jpg O=ours2}} &
\raisebox{-0.5\height}{\includegraphics[width=0.45\linewidth]{http://people.ee.ethz.ch/~mentzerf/pix2bits_results/bpg/kodak_bpg/kodim02_bpg_45_0.0313.png O=bpg2}}&
\rotatebox[origin=c]{90}{BPP3 bpp}\vspace{2pt} \\
\rotatebox[origin=c]{90}{BPP4 bpp}&
\raisebox{-0.5\height}{\includegraphics[width=0.45\linewidth]{https://people.ee.ethz.ch/~aeirikur/pix2bits_results/openimages_GC_60ch_NL_MSE10_BN4_LEVELS5no_IN200918_kodakperchannel/test_iter_140000/images/kodim03_0.03424bpp_synthesized_image.jpg O=ours3}} &
\raisebox{-0.5\height}{\includegraphics[width=0.45\linewidth]{http://people.ee.ethz.ch/~mentzerf/pix2bits_results/bpg/kodak_bpg/kodim03_bpg_46_0.0347.png O=bpg3}}&
\rotatebox[origin=c]{90}{BPP5 bpp}\vspace{2pt} \\
\rotatebox[origin=c]{90}{BPP6 bpp}&
\raisebox{-0.5\height}{\includegraphics[width=0.45\linewidth]{https://people.ee.ethz.ch/~aeirikur/pix2bits_results/openimages_GC_60ch_NL_MSE10_BN4_LEVELS5no_IN200918_kodakperchannel/test_iter_140000/images/kodim04_0.03241bpp_synthesized_image.jpg O=ours4}} &
\raisebox{-0.5\height}{\includegraphics[width=0.45\linewidth]{http://people.ee.ethz.ch/~mentzerf/pix2bits_results/bpg/kodak_bpg/kodim04_bpg_48_0.0322.png O=bpg4}}&
\rotatebox[origin=c]{90}{BPP7 bpp}\vspace{2pt} \\
\rotatebox[origin=c]{90}{BPP8 bpp}&
\raisebox{-0.5\height}{\includegraphics[width=0.45\linewidth]{https://people.ee.ethz.ch/~aeirikur/pix2bits_results/openimages_GC_60ch_NL_MSE10_BN4_LEVELS5no_IN200918_kodakperchannel/test_iter_140000/images/kodim05_0.03552bpp_synthesized_image.jpg O=ours5}} &
\raisebox{-0.5\height}{\includegraphics[width=0.45\linewidth]{http://people.ee.ethz.ch/~mentzerf/pix2bits_results/bpg/kodak_bpg/kodim05_bpg_50_0.0816.png O=bpg5}}&
\rotatebox[origin=c]{90}{BPP10 bpp}\vspace{2pt} \\
\end{tabular}}
