# Supplementary material for: Generative Adversarial Networks for Extreme Learned Image Compression
Source: arXiv:1804.02958 source file (2019-08-18)
Supplement: Supplementary file 3 [file fig_appendix_raise1k_base.tex]

OUTDIR=fig_appendix_raise1k
{\setlength{\tabcolsep}{1pt}
\begin{tabular}{rccl}
&Ours&BPG\\
\rotatebox[origin=c]{90}{BPP0 bpp}&
\raisebox{-0.5\height}{\includegraphics[width=0.45\linewidth]{https://people.ee.ethz.ch/~aeirikur/pix2bits_results/openimages_GC_60ch_NL_MSE10_BN4_LEVELS5no_IN240918_raise1k_768_max_eirikurperchannel/test_iter_140000/images/r01cbb7fdt_0.03551bpp_synthesized_image.jpg O=ours1}} &
\raisebox{-0.5\height}{\includegraphics[width=0.45\linewidth]{https://data.vision.ee.ethz.ch/mentzerf/user_study_extreme/raise1k_768_ae/r01cbb7fdt_bpg_50_0.0380.png O=bpg1}}&
\rotatebox[origin=c]{90}{BPP1 bpp}\vspace{2pt} \\
\rotatebox[origin=c]{90}{BPP2 bpp}&
\raisebox{-0.5\height}{\includegraphics[width=0.45\linewidth]{https://people.ee.ethz.ch/~aeirikur/pix2bits_results/openimages_GC_60ch_NL_MSE10_BN4_LEVELS5no_IN240918_raise1k_768_max_eirikurperchannel/test_iter_140000/images/r03640e97t_0.03531bpp_synthesized_image.jpg O=ours2}} &
\raisebox{-0.5\height}{\includegraphics[width=0.45\linewidth]{https://data.vision.ee.ethz.ch/mentzerf/user_study_extreme/raise1k_768_ae/r03640e97t_bpg_51_0.0530.png O=bpg2}}&
\rotatebox[origin=c]{90}{BPP3 bpp}\vspace{2pt} \\
\rotatebox[origin=c]{90}{BPP4 bpp}&
\raisebox{-0.5\height}{\includegraphics[width=0.45\linewidth]{https://people.ee.ethz.ch/~aeirikur/pix2bits_results/openimages_GC_60ch_NL_MSE10_BN4_LEVELS5no_IN240918_raise1k_768_max_eirikurperchannel/test_iter_140000/images/r04cfa379t_0.03422bpp_synthesized_image.jpg O=ours3}} &
\raisebox{-0.5\height}{\includegraphics[width=0.45\linewidth]{https://data.vision.ee.ethz.ch/mentzerf/user_study_extreme/raise1k_768_ae/r04cfa379t_bpg_50_0.0378.png O=bpg3}}&
\rotatebox[origin=c]{90}{BPP5 bpp}\vspace{2pt} \\
\rotatebox[origin=c]{90}{BPP6 bpp}&
\raisebox{-0.5\height}{\includegraphics[width=0.45\linewidth]{https://people.ee.ethz.ch/~aeirikur/pix2bits_results/openimages_GC_60ch_NL_MSE10_BN4_LEVELS5no_IN240918_raise1k_768_max_eirikurperchannel/test_iter_140000/images/r066ef803t_0.03596bpp_synthesized_image.jpg O=ours4}} &
\raisebox{-0.5\height}{\includegraphics[width=0.45\linewidth]{https://data.vision.ee.ethz.ch/mentzerf/user_study_extreme/raise1k_768_ae/r066ef803t_bpg_51_0.0444.png O=bpg4}}&
\rotatebox[origin=c]{90}{BPP7 bpp}\vspace{2pt} \\
\rotatebox[origin=c]{90}{BPP8 bpp}&
\raisebox{-0.5\height}{\includegraphics[width=0.45\linewidth]{https://people.ee.ethz.ch/~aeirikur/pix2bits_results/openimages_GC_60ch_NL_MSE10_BN4_LEVELS5no_IN240918_raise1k_768_max_eirikurperchannel/test_iter_140000/images/r0809811bt_0.03399bpp_synthesized_image.jpg O=ours5}} &
\raisebox{-0.5\height}{\includegraphics[width=0.45\linewidth]{https://data.vision.ee.ethz.ch/mentzerf/user_study_extreme/raise1k_768_ae/r0809811bt_bpg_47_0.0391.png O=bpg5}}&
\rotatebox[origin=c]{90}{BPP10 bpp}\vspace{2pt} \\
\end{tabular}}
